# Supplementary material for: Color: A Framework for Applying Graph Coloring to Subgraph Cardinality Estimation
Source: arXiv:2405.06767 source file (2025-04-29)
Supplement: Supplementary file 1 [file appendix.tex]

\begin{appendix}
\section{Proof of Thm. \ref{thm:stable-colorings}}
\label{app:proof-stable-colorings}
In this section, we prove the following theorem for simple graphs, but the extension to property graphs is straightforward.
\begin{thm}
Let $\calG$ be a lifted graph defined by a stable coloring $\sigma$. Then $\tau_{\text{min}}=\tau_{\text{avg}}=\tau_{\text{max}}$, and, for any acyclic query $Q$, the lifted graph estimator is exact:
\begin{align}
  |\hom(Q,G)| = \Phi(Q, \calG)
\end{align}
\end{thm}

\begin{proof}
We start by noting that each match in the data graph, $\pi \in Hom(Q, G)$, is associated with precisely one coloring, $\pi'\in Hom(Q,F)$, based on the matched vertices' colors, i.e. $\pi' = \sigma_S \circ \pi $. We denote the set of matches with this coloring as $Hom(Q,G |\pi')$. If we calculate $|Hom(Q,G|\pi')|$ for each coloring, $\pi'$, then we can compute the total as $\sum_{\pi'\in Hom(Q,F)}|Hom(Q,G|\pi')|$. By this logic and equation \ref{eq:standard-estimator}, we simply need to show that $W(\pi') = |Hom(Q,G|\pi')|$.

We note that $Q$ is a acyclic and proceed inductively on the topological ordering $v_1,\ldots,v_{|Q|}$. Let $Q_i$ be the sub-tree restricted to the vertices $v_1,\ldots,v_i$, and let $\pi'_i$ be the coloring restricted to these vertices. We begin with the base case,
\begin{align*}
    W(\pi'_1) = \psi(\pi'_1(v_1)) = |Hom(Q_1,G|\pi'_1)|
\end{align*}
The number of matches to a vertex of a color is equal to the number of vertices in that color, so this is immediately true. Now, suppose that $W(\pi'_i) = |Hom(Q_i,G|\pi'_i)|$, and we will show that $W(\pi'_{i+1}) = |Hom(Q_{i+1},G|\pi'_{i+1})|$. We restate Eq. \ref{eq:standard-estimator} as follows,
\begin{align*}
    W(\pi'_{i+1}) = \psi(\pi'_{i+1}(v_1)) \prod_{(v_j,v_k)\in E_{Q_{i+1}}} \tau((\pi'_{i+1}(v_j),\pi'_{i+1}(v_k)))
\end{align*}
Let $v_j$ be the parent of $v_{i+1}$, and we can express $W_{\psi, \tau}(\pi'_{i+1})$ inductively,
\begin{align*}
W(\pi'_{i+1}) = W(\pi'_i) \cdot \tau((\pi_{i+1}(v_j),\pi_{i+1}(v_{i+1})))    
\end{align*}
By our inductive assumption, this means,
\begin{align*}
W(\pi'_{i+1}) = |Hom(Q_i, G|\pi'_i)|\cdot \tau((\pi_{i+1}(v_j),\pi_{i+1}(v_{i+1})))    
\end{align*}
Denote the number of edges that a vertex $v\in V_G$ has to vertices with color $C$ as $deg_G(v|C)$. Because $\sigma_S$ is a stable coloring, we know,
\begin{align*}
deg_G(v|C) = deg_G(v'|C) \,\,\,\forall v,v'\in V_G \,\, s.t.\,\,\sigma_S(v)=\sigma_S(v')
\end{align*}
By the definition of $\tau$, this degree is precisely,
\begin{align*}
deg_G(v|C) = \tau(\sigma_S(v_j), C)
\end{align*}
We denote this degree with its color as $deg_G(C|C')$. Returning to our expression for $W_{\psi, \tau}(\pi'_{i+1})$, we can now plug in our degree expression,
\begin{align*}
W(\pi'_{i+1}) &= |Hom(Q_i,G|\pi'_i)|\cdot deg_G(\pi'_{i+1}(v_j)|\pi'_{i+1}(v_{i+1}))\\
\end{align*}
By simply expanding $|Hom(Q_i,G|\pi'_i)|$ into a sum, we get,
\begin{align}
\label{app:eq:induction}
W^{std}(\pi'_{i+1}) &= \sum_{\pi_i\in Hom(Q_i,G|\pi'_i)} deg_G(\pi'_{i+1}(v_j)|\pi'_{i+1}(v_{i+1}))
\end{align}
At this point, we use the fact that $deg(\pi'_i(v_j)|\pi'_{i+1}(v_{i+1}))$

$ = deg(\pi_i(v_j)|\pi'_{i+1}(v_{i+1}))$ when $\sigma_S(\pi_i(v_j)) = \pi'_i(v_j)$,  which is assured by $\pi\in Hom(Q_i,G|\pi'_i)$.  
\begin{align}
\label{app:eq:inductive_goal}
W^{std}(\pi'_{i+1}) &= \sum_{\pi_i\in Hom(Q_i,G|\pi'_i)} deg_G(\pi_{i}(v_j)|\pi'_{i+1}(v_{i+1}))
\end{align}

Because $Q$ is a tree, the RHS is the target of the induction,
$$W^{std}(\pi'_{i+1}) = |Hom(Q_{i+1},G|\pi'_{i+1})|$$

To prove the corollary, we reconsider Eq.~\eqref{app:eq:induction} in the case of quasi-stable or approximate colorings. We know that the maximum degree of a node in the color $\pi'_{i+1}(v_j)$ to another color $\pi'_{i+1}(v_{i+1})$ is at most $\epsilon$ times greater than the minimum degree. Therefore, the relative error between the true degree, $deg(\pi_i(v_j)|\pi'_{i+1}(v_{i+1}))$ and the average degree, $\tau(\pi'_{i+1}(v_j)|\pi'_{i+1}(v_{i+1}))$ must also be less than $\epsilon$. Because each term in the sum on the RHS of Eq.~\eqref{app:eq:induction} is within $\epsilon$ of the true degree for each node, the total sum must be only an $\epsilon$ multiplicative factor from the true in the RHS of ~\eqref{app:eq:inductive_goal}. Lastly, we note that each step of our inductive proof only incurs an $\epsilon$ relative error, so the entire result must be within the desired $\epsilon^{(|Q|-1)}$ relative error.

\end{proof}

\section{Proof of Theorem \ref{thm:inference-tw}}
We begin by restating the theorem,
\begin{thm}
Given a query graph, $Q$, a lifted graph, $F$, and a decomposable estimator $W$, $\Phi(Q, F, W_{\psi, \tau})$ can be computed in time $O(|C|^{tw(Q)})$ where $tw(Q)$ is the treewidth of $Q$ where $\Phi(Q,F,W_{\psi, \tau})$ is defined,
\begin{align*}
        \Phi(Q, F, W_{\psi, \tau}) = \sum_{c_{v_1},...,c_{v_{|Q|}}\in C} \psi(c_0)\prod_{i=1}^{|E_Q|}\omega(\pi_{v_k\rightarrow c_{v_k}},e_i|e_1,...,e_{i-1})
\end{align*}
\end{thm}

We now define tree decompositions,
\begin{definition}
    Given a graph $H$, a tree decomposition $T(E_T, V_T, \chi, \gamma)$ is composed of four pieces,
    \begin{enumerate}
        \item $E_T$, $V_T$ are the edges and vertices of a tree
        \item $\chi: V_T \rightarrow 2^{V_H}$ is a function which maps vertices in the tree to sets of vertices in $H$
        \item $\gamma: V_T \rightarrow 2^{E_H}$ is a function which maps vertices in the tree to sets of edges in $H$
    \end{enumerate}
    Lastly, it has two requirements,
\begin{enumerate}
    \item For all $v\in V_H$, the set of vertices in $V_T$ that contain $v$ form a connected sub-tree
    \item Each edge in $E_H$ is mapped to exactly one vertex of $V_T$ by $\gamma$ and the vertex of $V_T$ which it is mapped to includes both the endpoints
\end{enumerate}     
\end{definition}
The treewidth is then defined as follows,
\begin{definition}
    Given a graph $H$, let the set of valid tree decompositions be $\mathcal{T}_H$. The treewidth is then defined as,
    \begin{align*}
        \min_{T\in\mathcal{T}_H}\max_{v\in V_T} |\chi(v)| - 1
    \end{align*}
\end{definition}
Intuitively, graphs that are "more acyclic" will have a lower treewidth and graphs that are "more cyclic" have a higher treewidth. 

\begin{proof}
For this problem, we can take advantage of tree decompositions by using them to structure the summation in \eqref{eq:optimization:faq_version}. Suppose that the treewidth of $Q$ is $k$ and let $T(E_T, V_T, \chi)$ be a tree decomposition which matches this width. To avoid confusion, we will denote vertices of $T$ as $v_i'$ and vertices of $Q$ as $v_i$. Further, let $v_1', \cdots, v_{|V_T|}'$ be a topological ordering of $T$ where $v_1'$ is the root of the tree, and let $v_1, \cdots, v_{|V_Q|}$ be an ordering of $Q$ such that the sub-tree corresponding to $v_i$ is not a sub-tree of $v_{>i}$. Let $Par(v')$ denote the parent of $v'$ in $T$ and let $Ch(v')$ be the set of child vertices of $v'$ in $T$. Lastly, we denote the set of query vertices which associated with $v_{|V_T|}'$ and not its parent as $\mathbf{X}_{i} = \chi(v_i') \setminus \chi(Par(v_i'))$. We denote the set of query vertices which are associated with $v_{|V_T|}'$ AND its parent as $\mathbf{Y}_{|V_T|} =  \chi(v_{|V_T|}') \cap \chi(Par(v_{|V_T|}'))$.

We will proceed iteratively on these vertices starting with $v_{|V_T|}'$ and proceeding backwards towards the root. 

\textbf{Base Case:} Our base case is $v_{|V_T|}'$ which is necessarily a leaf of the true due to the topological ordering. 
We denote the output of the base case as the function $S_{|V_T|}(c_{y_1},\ldots,c_{y_m})$ and define it as follows,
\begin{align*}
    S_{|V_T|}(c_{y_1},\ldots,c_{y_m}) = \sum_{c_{x_1},\ldots,c_{x_n}\in C} \prod_{e_i\in \gamma(v_{|V_T|}')} \omega(\pi_{x_j\rightarrow c_{x_j}}, e_i | e_1,\ldots,e_{i-1})
\end{align*}
At this point of the computation, we will fully materialize the values of the function $S_{|V_T|}$ which has a domain of size $|C|^{|Y_{|V_T|}|}$ and each point requires computing a summation of $|C|^{|X_{|V_T|}|}$ terms. Therefore, the entire computation requires $|C|^{|\chi(v_{|V_T|}')|} \leq |C|^k$ time.

\textbf{Inductive Case:} Suppose that all vertices $v_{j}'$ where $j>i$ have already been processed, we now consider handling $v_i'$. The output of this step is defined as,
\begin{align*}
    S_{i}(c_{Y_{v_i',1}},\ldots,c_{Y_{v_i',m}}) = \sum_{c_{X_{v_i',1}},\ldots,c_{X_{v_i',n}}\in C} & \prod_{e_i\in \gamma(v_i')} \omega(\pi_{X_{v_i',j}\rightarrow c_{X_{v_i',j}}}, e_i | e_1,\ldots,e_{i-1})\cdot\\
    &\prod_{v_j' \in Ch(v_i')} S_{v_j'}(c_{Y_{v_j', 1}},\ldots,c_{Y_{v_j', m}})
\end{align*}
As in the base case, the computation required to fully materialize the values of $S_i$ is bounded by $|C|^{|\chi(v_{|V_T|}')|} \leq |C|^k$. 

At this point, we just need to confirm that $S_1$ is equal to $\Phi(Q, F, W_{\psi,\tau})$ by showing that the sequence of computations represents a valid rearrangement of the sums of the original formula. To this end, we note that every query vertex appears in the summation of precisely one inductive step. This is due to the fact that each query vertex forms a sub-tree in the tree decomposition, so the root of that sub-tree is the only tree vertex which contains it and whose parent does not. Further, each instance of $\omega(\pi_{X_{v_i',j}\rightarrow c_{X_{v_i',j}}}, e_i | e_1,\ldots,e_{i-1})$ occurs precisely once because of the requirement that each edge of the query graph occurs in one vertex of the tree decomposition.

\end{proof}

\end{appendix}
